# Supplementary material for: Traveling fronts in active-passive particle mixtures
Source: arXiv:1601.00850 ancillary file (2016-01-05)
Supplement: Supplementary file 1 [file SI.pdf]

# Supplementary Materials for "Travelling fronts in active-passive particle mixtures."

Adam Wysocki, Roland G. Winkler, Gerhard Gompper[1]

[1] *Theoretical Soft Matter and Biophysics,*

*Institute of Complex Systems and Institute for Advanced Simulation,*

*Forschungszentrum Jülich, 52425 Jülich, Germany*

(Dated: January 5, 2016)

## MOVIES

- bulk_segregation_order.mp4 – Segregation order parameter field $\Phi(\mathbf{r})$ (color-coded) and the interface positions (black lines). Steady state system of size $L_x = L_y = 400$ with $N = 160000$ particles of a phase-separated active-passive mixture ($x_A = 0.5$). The movie corresponds to Fig. 1(a,b) of the main text.

- Phase-separated active-passive mixture ($x_A = 0.5$) with propagating interfaces in an elongated box (one advancing, the other receding). Interface positions are indicated by dashed lines. The movies correspond to Fig. 2(a-c) of the main text.
  - positions_mixture.mp4 – Positions of active (red) and passive (blue) particles.
  - vorticity_mixture.mp4 – Vorticity and particle flux field.
  - mixing_mixture.mp4 – Visualisation of mixing. Initially particles are colored according to their $x$ position (indicated by the color scale).

- Phase-separated pure active fluid ($x_A = 1$) with non-propagating interfaces in an elongated box. The movies correspond to Fig. 1(a-c) of the SI text.
  - positions_pure.mp4 – Particle positions.
  - vorticity_pure.mp4 – Vorticity and particle flux field.
  - mixing_pure.mp4 – Visualisation of mixing.

## COARSE-GRAINED FIELDS

The coarse-grained packing density fields $\phi_\alpha(\mathbf{r})$ of active ($\alpha = A$) and passive ($\alpha = P$) particles at position $\mathbf{r} = (x, y)$ are defined as

$$\phi_\alpha(\mathbf{r}) = \frac{\pi}{4}\left[\sum_{i=1}^{N_\alpha} f(\mathbf{r}-\mathbf{r}_i)\right], \tag{1}$$

where $f(\mathbf{R}) = \exp\left[-|\mathbf{R}|^2/(2w^2)\right]/(2\pi w^2)$ is a Gaussian coarse-graining function and $w$ is a coarse-graining scale [1]; we employ $w = 2$ or $w = 3$. Hence, we obtain the segregation order parameter field as

$$\Phi(\mathbf{r}) = (\phi_A - \phi_P)/(\phi_A + \phi_P). \tag{2}$$

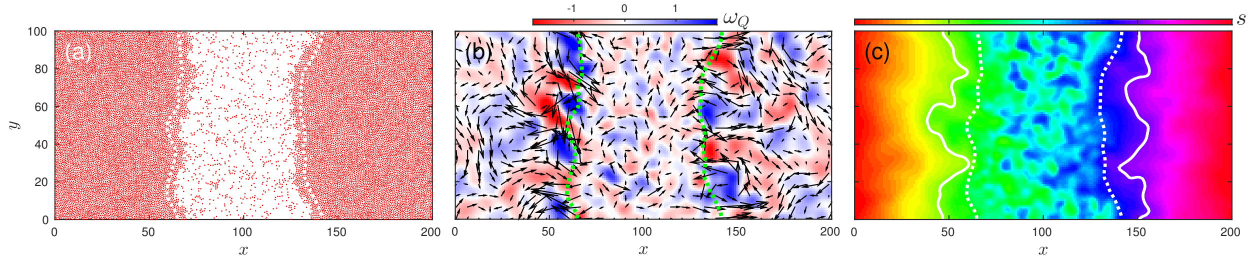


FIG. 1. (color online) (a) Snapshot of an one-component active Brownian discs fluid ($x_A = 1$) in a box of size $L_x = 100$ and $L_y = 200$. The interface positions are indicated by dashed lines. (b) Vorticity $\omega_Q(\mathbf{r}) = \nabla \times \mathbf{Q}(\mathbf{r})$, where $\mathbf{Q}$ is the coarse-grained particle flux [Eq. (3)]. (c) Visualisation of the bulk flow. Particle positions are shown after the time lag $\delta t = 1$, where particles are colored according to their initial $x$ position, as indicated by the color scale [Eq. (4)]. The solid lines mark the isolines of $s(\mathbf{r}, \delta t)$ used for the stability analysis.

The vorticity $\omega_Q(\mathbf{r}) = \nabla \times \mathbf{Q}(\mathbf{r})$ is obtained from the coarse-grained particle flux

$$\mathbf{Q}(\mathbf{r}, t) = \sum_{i=1}^{N} \mathbf{v}_i(t) f(\mathbf{r} - \mathbf{r}_i(t)), \tag{3}$$

where $\mathbf{v}_i(t) = \frac{\mathbf{r}_i(t+\delta t) - \mathbf{r}_i(t)}{\delta t}$ is the microscopic velocity of the $i$th particle with time lag $\delta t = 0.4$.

In order to visualize the mass transport in the elongated box of Fig. 2 in the main text and of Fig. 1 in the SI text, we construct a scalar displacement field (related to a passive scalar field normally used to study fluid mixing [2]) using the horizontal positions $x_i(t)$ of all particles $i$ at time $t$ according to

$$s(\mathbf{r}, \delta t) = \frac{\sum_{i=1}^{N} x_i(t) f(\mathbf{r} - \mathbf{r}_i(t + \delta t))}{\sum_{i=1}^{N} f(\mathbf{r} - \mathbf{r}_i(t + \delta t))}. \tag{4}$$

## INTERFACE POSITION

We use a robust and unbiased approach to define the interface position $\mathbf{r}_I$ between the dense and the dilute phase by choosing an isoline of the overall packing density field, i.e., we set $\phi(\mathbf{r}_I) = \phi_A(\mathbf{r}_I) + \phi_P(\mathbf{r}_I) = \phi_I$. A phase-separated system exhibits a bimodal distribution of the local packing fraction and basically any value in the range spanned by the two characteristic packing fractions could be used for $\phi_I$; we choose $\phi_I = 0.8$, a value close to the high density peak. The choice of $w$ does not affect the interface properties on length

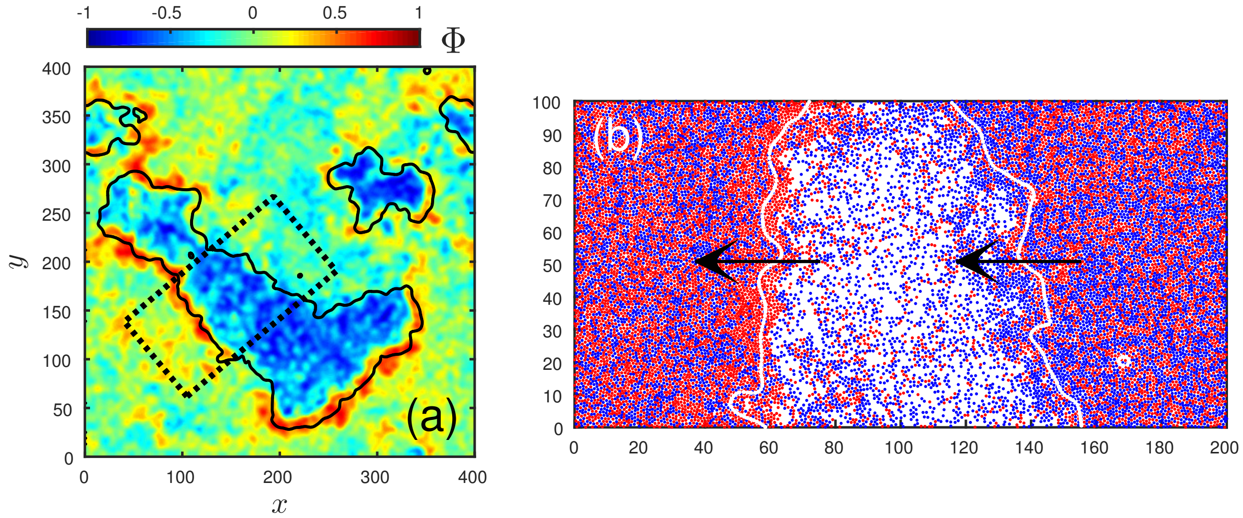


FIG. 2. (color online) (a) Snapshot of the segregation order parameter field $\Phi(\mathbf{r})$ [Eq. (2)] of a system of size $L_x = L_y = 400$ in the steady state at $x_A = 0.5$. $\Phi = 1$ ($\Phi = -1$) corresponds to a pure active (passive) phase and $\Phi = 0$ corresponds to a uniform mixture. The black line indicates the interface position. The corresponding movie is `bulk_segregation_order.mp4`. (b) Closeup of a region with in parallel propagating fronts [indicated by a dashed frame in (a)]. The positions of active and passive particles are marked by red and blue dots, respectively.

scales larger then $w$. It is useful to note that in equilibrium fluids, an instantaneous Gibbs dividing surface is mostly used to construct an interface position [3].

## DISCUSSION OF FIG. 2

In a quasi-one-dimensional simulation box interfaces propagate in pairs, namely, an advancing together with a receding interface. This might not be the case in a large square simulation box, where both types of interfaces (advancing and receding) may propagate independently of each other, as can be seen in the movie corresponding to Fig. 2(a) of the SI text. Nevertheless, a pairwise propagation of interfaces occur quite frequently in a large square simulation box as is illustrated in Fig. 2(b), where a closeup of a region with in parallel propagating fronts is shown.


[1] I. Goldhirsch, Granular Matter **12**, 239 (2010).

[2] D. Saintillan and M. J. Shelley, Phys. Fluids **20**, 123304 (2008).

[3] R. L. C. Vink, J. Horbach, and K. Binder, J. Chem. Phys. **122**, 134905 (2005).
